# Supplementary material for: Universal critical behavior in the ferromagnetic superconductor Eu(Fe$_{0.75}$Ru$_{0.25}$)$_{2}$As$_{2}$
Source: arXiv:1904.07417 source file (2019-08-15)
Supplement: Supplementary file 1 [file SM_Eu_v10_revised.pdf]

# Supplemental Material for

## Universal critical behavior in the ferromagnetic superconductor

### $\text{Eu}(\text{Fe}_{0.75}\text{Ru}_{0.25})_2\text{As}_2$

W. T. Jin<sup>1,\*,\dagger</sup>, Zheng Zhou<sup>2,\*</sup>, Wei Li<sup>2,3,\*,\ddagger</sup>, S. Nandi<sup>4</sup>, B. Ouladdiaf<sup>5</sup>, Zheng Yan<sup>2,\S</sup>, Xinyuan Wei<sup>2</sup>, Xuguang Xu<sup>6</sup>, W. H. Jiao<sup>7</sup>, N. Qureshi<sup>5</sup>, Y. Xiao<sup>8</sup>, Y. Su<sup>1</sup>, G. H. Cao<sup>9</sup>, Th. Brückel<sup>4,1</sup>

<sup>1</sup> Jülich Centre for Neutron Science JCNS at Heinz Maier-Leibnitz Zentrum (MLZ), Forschungszentrum Jülich GmbH, Lichtenbergstraße 1, D-85747 Garching, Germany

<sup>2</sup> State Key Laboratory of Surface Physics and Department of Physics, Fudan University, Shanghai 200433, China

<sup>3</sup> Collaborative Innovation Center of Advanced Microstructures, Nanjing 210093, China

<sup>4</sup> Jülich Centre for Neutron Science JCNS and Peter Grünberg Institut PGI, JARA-FIT, Forschungszentrum Jülich GmbH, D-52425 Jülich, Germany

<sup>5</sup> Institut Laue Langevin, 71 rue des Martyrs, BP156, 38042 Grenoble Cedex 9, France

<sup>6</sup> School of Physical Science and Technology, ShanghaiTech University, Shanghai 201210, China

<sup>7</sup> School of Science, Zhejiang University of Science and Technology, Hangzhou 310023, China

<sup>8</sup> School of Advanced Materials, Peking University Shenzhen Graduate School, Shenzhen 518055, China

<sup>9</sup> Department of Physics, Zhejiang University, Hangzhou 310027, China

\*These authors contributed equally to this work.

Correspondence to: <sup>\dagger</sup> W.T.J (jwt2006@gmail.com); <sup>\ddagger</sup> W.L. (W\_Li@fudan.edu.cn); <sup>\S</sup> Z.Y. (zhengyan13@fudan.edu.cn)

#### **This PDF file includes:**

Supplementary Text

Table S1

Figs. S1

References (1-11)

#### A. Experimental details of the neutron diffraction and resistivity measurements

The crystal was mounted on top of an aluminum pin with a tiny amount of GE varnish and put inside a closed-cycle cryostat in the four-circle geometry. A Cu (2 0 0) monochromator was used to produce a monochromatic neutron beam with the wavelength of 1.26 Å. An area detector was used for collecting the integrated intensities of accessible reflections, and a flat pyrolytic graphite PG (0 0 8) analyzer was used to reduce the background when searching for weak reflections and performing reciprocal-space scans. The electric resistivity of the same piece of crystal was measured using a Quantum Design physical property measurement system.

#### B. Summary of the universal critical exponent values of $\beta$ for the ferromagnetic theoretical models.

In this section, we mainly summarize the universal critical exponent values of  $\beta$  for some basic theoretical models for describing the ferromagnetism in condensed matter physics, including the three-dimensional (3D) and two-dimensional (2D) Ising model, as well as the 2D and 3D classical and quantum Heisenberg models, as listed in Table S1. From those values of  $\beta$ , we notice that the higher dimensionality of systems are, the larger values of critical exponent values of  $\beta$  will be. It suggests that the critical exponent value of  $\beta$  will be enhanced gradually as increasing the number of bonding. In addition, comparing with the critical exponent values of  $\beta$  for the classical and the quantum Heisenberg modes, the infinity limit of multiple degrees of freedom in spin favors to significantly enhance the critical exponent values of  $\beta$ .

TABLE S1: Summary of the universal critical exponent values of  $\beta$  for some basic ferromagnetic theoretical models.

| Theoretical Model       | $\beta$ value | References |
|-------------------------|---------------|------------|
| 3D quantum Heisenberg   | 0.365         | Ref [1]    |
| 2D quantum Heisenberg   | 0.35          | Ref [2]    |
| 3D classical Heisenberg | 0.693         | Ref [3]    |
| 2D classical Heisenberg | 0.5           | Ref [4]    |
| 3D Ising                | 0.3258        | Ref [5]    |
| 2D Ising                | 0.125         | Ref [6]    |

#### B. Evaluating the magnetic exchange coupling for the ferromagnetic superconductor $\text{Eu}(\text{Fe}_{0.75}\text{Ru}_{0.25})_2\text{As}_2$ based on the first-principles calculations.

The magnetic behavior for Eu spins is described as following theoretical model,

$$\hat{H} = J_1 \sum_{\langle i,j \rangle} \vec{S}_i \vec{S}_j + J_2 \sum_{\langle\langle i,j \rangle\rangle} \vec{S}_i \vec{S}_j + J_{\perp} \sum_{\langle i,j \rangle} \vec{S}_i \vec{S}_j, \quad (\text{S1})$$

where  $\vec{S}_i$  is the magnitude of Eu spin on the site  $i$ ,  $\langle i, j \rangle$  and  $\langle\langle i, j \rangle\rangle$  denoting the summation over the nearest neighbor and next-nearest neighbor sites, respectively. The parameters  $J_1$  and  $J_2$  describe the nearest neighboring and next-nearest neighboring intralayer exchange interactions.  $J_{\perp}$

denotes the nearest neighboring interlayer exchange interaction. The interlayer magnetic exchange coupling constant  $J_{\perp}$  can be evaluated through the configurations of A-type antiferromagnetic ( $E_{AFM}$ ) and ferromagnetic ( $E_{FM}$ ) orders [7]. The obtained coupling constant is

$$J_{\perp} = \frac{1}{16} (E_{FM} - E_{AFM}) = -0.49 \text{ meV}.$$

Furthermore, the in-plane magnetic exchange coupling constants of  $J_1$  and  $J_2$  can be evaluated through the four states configurations based on the  $2 \times 2$  supercell method [8, 9],

$$J_{1,2} = \frac{E_{\uparrow\uparrow} + E_{\downarrow\downarrow} - E_{\uparrow\downarrow} - E_{\downarrow\uparrow}}{4S^2}, \quad (S2)$$

and we thus obtain that the values of magnetic exchange coupling for  $J_1$  and  $J_2$  are -4.1 meV and 0.51 meV, respectively.

### C. Detailed quantum Monte Carlo calculations for the evaluation of critical exponent value $\beta$ for the ferromagnetic superconductor $\text{Eu}(\text{Fe}_{0.75}\text{Ru}_{0.25})_2\text{As}_2$ .

The stochastic series expansion (SSE) algorithm with operator loop updated [10] is used to evaluate the exact value of critical exponent  $\beta$ . In the following we make a brief introduction to the SSE method. The exponential operator in the partition function  $Z = \text{Tr } e^{\beta' \hat{H}}$  is taken care of by a Taylor expansion and the trace is described by the summation over a complete set of states in a suitable-chosen basis in the Monte Carlo algorithm:

$$Z = \sum_{\alpha} \sum_{n=0}^{+\infty} \frac{\beta'^n}{n!} \langle \alpha | (-\hat{H})^n | \alpha \rangle \quad (S3)$$

where  $|\alpha\rangle$  is a randomly chosen state and  $\beta' = 1/k_B T$ .  $k_B$  is the Boltzmann constant and  $T$  is the temperature. Then the Hamiltonian  $\hat{H}$  shown in Eq. S1 is rewritten as the summation of a set of operators whose matrix elements can be conveniently obtained. We thus stochastically pick configurations from such infinite summation by means of importance sampling and average the observables over the states  $|\alpha\rangle$ .

Since the calculated next-nearest neighbor magnetic coupling  $J_2 = 0.51 \text{ meV}$  is antiferromagnetic, it makes the sign problem in the quantum Monte Carlo algorithm, where the sign problem refers to the emergence of negative weights. Fortunately, the next-nearest neighbor antiferromagnetic exchange coupling  $J_2 = 0.51 \text{ meV}$  is much smaller compared to the nearest neighbor ferromagnetic exchange coupling  $J_1 = -4.1 \text{ meV}$ , this sign problem can be dealt as simplify by the following technique, that the expectation value of the observables can be rewritten as

$$\langle O \rangle = \frac{\sum_i W_i O_i}{\sum_i W_i} = \frac{\sum_i W_i O_i / \sum_i |W_i|}{\sum_i W_i / \sum_i |W_i|} = \frac{\langle O \text{sgn } W \rangle'}{\langle \text{sgn } W \rangle'} \quad (S4)$$

where  $W_i$  is the weights of the samplings, some of the  $W_i$ 's might be negative. We replace the negative weights by its absolute value  $|W_i|$ , the expectation value measured in these new weights are thus denoted by  $\langle \cdot \rangle'$ . We measure the expectation value of the observables and the sign of the weights simultaneously. Their quotient is the expectation in original weights.

In the practical numerical calculations, we carry out the calculations for various  $L \times L \times L$  cubes with  $L = 8$  to  $14$ . We set the number of bins to be  $50$ , the first  $10$  for reaching thermodynamic balance and the rest ones to measure physical observables. Each bin contains  $1000$  Monte Carlo steps.

We measured the magnetization  $m$  and its reduced four order Binder cumulant  $U$  for different system scales  $L$ . the Binder cumulant reaches  $1$  at orderless phase and reaches  $0$  at ordered phase. The observables are defined as following:

$$m = \langle \sum_i S_i^z \rangle \quad (S5)$$

$$U = 3 \left( 1 - \frac{1}{2} \frac{\langle m^4 \rangle}{\langle m^2 \rangle^2} \right) \quad (S6)$$

The finite size scaling [11] proposes that these quantities should behave as

$$m_L(T) = L^{-\beta/\nu} \bar{m}(L^{1/\nu} \tau) \quad (S7)$$

$$U_L(T) = \bar{U}(L^{1/\nu} \tau) \quad (S8)$$

in vicinity of the critical point, where  $\tau = (T - T_c)/T_c$  and  $\bar{U}$  and  $\bar{m}$  are universal functions that are independent on the scale of  $L$ . The parameter  $\nu$  is also a critical exponent, which describes the behavior of the correlation length in vicinity of the critical temperature. To improve the fitting result in Eq. S7, a correction of the form

$$m_L(T) = L^{-\beta/\nu} \bar{m}(L^{1/\nu} \tau) (1 + aL^{-\omega}) \quad (S9)$$

is introduced [12], where  $a$  and  $\omega$  are the correction parameters in the fittings. We use Binder cumulant  $U$  to determine the critical point since at the critical point  $U_L(T_c) = \bar{U}(0)$  that is independent on  $L$ . The result is obtained as

$$h_c = 1.0093. \quad (S10)$$

To obtain the critical exponent value of  $\beta$ , we have to deal with another exponent  $\nu$  as first. We make use of the relation of Eq. (S8) and work out the derivative  $dU/dT|_c$  at first for each length, the  $dU/dT|_c$  versus scale  $L$  relation should be linear and its slope gives  $1/\nu$ . The raw data, data collapse and the linear fitting are shown in Fig. S1(a), (c), and (e), respectively. Thus, we obtain the result

$$1/\nu = 1.347 \quad (S11)$$

Furthermore, the magnetization at critical temperature behaves as Eq. (S9). Therefore, the slope in  $\log m_c$  versus  $\log L$  relation gives the critical exponent  $-\beta/\nu$  (correction term considered). The raw data, data collapse and the fitting are shown in Fig. S1(b), (d), and (f), respectively. The obtained result is

$$\beta/\nu = 0.520 \quad (S12)$$

Finally, we obtain the critical exponent value

$$\beta = 0.386. \quad (S13)$$

This critical exponent value  $\beta = 0.386$  is quite in excellent agreement with our neutron scattering experimental observation of  $\beta = 0.385$  shown in the main text.

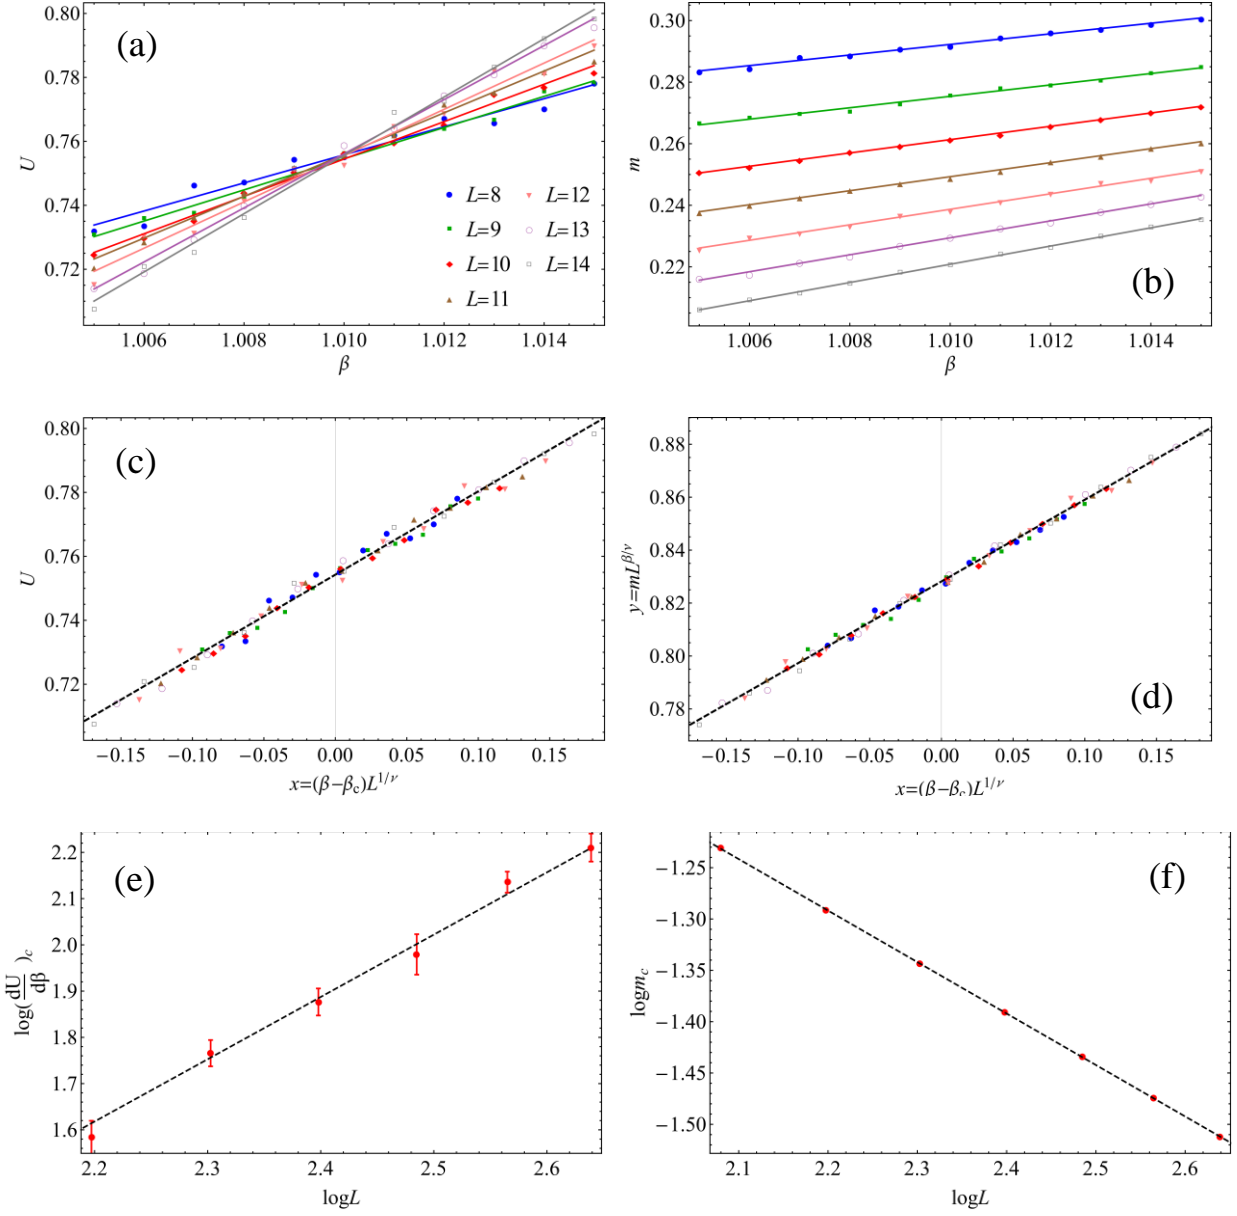

Fig. S1: (a) and (b) The raw data. (c) and (d) the data collapse for (a) and (c) Binder cumulant  $U$  and (b) and (d) magnetization  $m$ . The linear fitting whose slope gives (e)  $1/\nu$  and (f)  $\beta/\nu$ .

## References

1. L. Zhang, J. Fan, L. Li, R. Li, L. Ling, Z. Qu, W. Tong, S. Tan, and Yuheng Zhang, Critical properties of the 3D-Heisenberg ferromagnet  $\text{CdCr}_2\text{Se}_4$ , *Europhysics Letters* **91**, 57001 (2010).
2. Y. C. Chen, H. H. Chen, and F. Lee, Quantum Monte Carlo study of the spin-1/2 Heisenberg model, *Phys. Rev. B* **43**, 11082 (1991).
3. C. Holm and W. Janke, Critical exponents of the classical three-dimensional Heisenberg model: A single-cluster Monte Carlo study, *Phys. Rev. B* **48**, 936 (1993).
4. S. Fakioglu, Critical exponents for two-dimensional Heisenberg ferromagnet with long-range interaction, *Il Nuovo Cimento D* **10**, 1161 (1988).
5. A. M. Ferrenberg and D. P. Landau, Critical behavior of the three-dimensional Ising model: A high-resolution Monte Carlo study, *Phys. Rev. B* **44**, 5081 (1991).
6. C. N. Yang, The Spontaneous Magnetization of a Two-Dimensional Ising Model, *Phys. Rev.* **85**, 808 (1952).
7. W. Li, J.-X. Zhu, Y. Chen, and C. S. Ting, First-principles calculations of the electronic structure of iron-pnictide  $\text{EuFe}_2(\text{As,P})_2$  superconductors: Evidence for antiferromagnetic spin order, *Phys. Rev. B* **86**, 155119 (2012).
8. M.-H. Whangbo, H.-J. Koo, and D. Dai, Spin exchange interactions and magnetic structures of extended magnetic solids with localized spins: theoretical descriptions on formal, quantitative and qualitative levels, *Journal of Solid State Chemistry* **176**, 417 (2003).
9. H. J. Xiang, E. J. Kan, S.-H. Wei, M.-H. Whangbo, and X. G. Gong, Predicting the spin-lattice order of frustrated systems from first principles, *Phys. Rev. B* **84**, 224429 (2011).
10. A. W. Sandvik, Stochastic series expansion method with operator-loop update, *Phys. Rev. B* **59**, R14157 (1999).
11. V. Privman, Finite-Size Scaling and Numerical Simulation of Statistical Systems, *Singapore: World Scientific Singapore* (1990).
12. A. W. Sandvik., Computational Studies of Quantum Spin Systems, *AIP Conf. Proc.* **1297**, 135 (2010).
